# Supplementary material for: FLIP: Cross-domain Face Anti-spoofing with Language Guidance
Source: arXiv:2309.16649 source file (2023-09-28)
Supplement: Supplementary file 1 [file suppl_params.tex]

\begin{table}[t]
% \centering \small
\caption{Number of network parameters and computational complexity for all three methods in the FLIP framework.}
\label{tab:suppl_params}

\scalebox{0.85}[0.85]{
    \begin{tabular}{l|ccc|cc}
    \multicolumn{5}{c}{}\\
        \toprule
            \multirow{2}{*}{\textbf{Method}} & \multicolumn{2}{c}{\textbf{Training}} && \multicolumn{2}{c}{\textbf{Inference}}\\
                        & \textbf{Parameters} & \textbf{FLOPs} && \textbf{Parameters} & \textbf{FLOPs}\\
            \midrule
            FLIP-V          & 86.58M  & 17.58G  && 86.58M  & 17.58G\\
            FLIP-IT         & 150.00M & 23.55G  && 150.00M & 23.55G\\
            FLIP-MCL        & 170.00M & 23.58G && 150.00M & 23.55G \\
            \bottomrule
    \end{tabular}
}
\vspace{-1em}
\end{table}
